# Supplementary material for: Asymptotic preserving IMEX-DG-S schemes for linear kinetic transport equations based on Schur complement
Source: arXiv:2006.07497 source file (2020-06-12)
Supplement: Supplementary file 1 [file appendix.tex]

\appendix
\section{Butcher tableau for ARS($2,2,2$) and ARS($4,4,3$)}
\label{sec:appendix}
The double Butcher tableau of ARS($2,2,2$) and ARS($4,4,3$) schemes \cite{ascher1997implicit} are respectively
\begin{displaymath}
\begin{array}{c|c c c}
0 & 0&0&0\\
\gamma & \gamma&0&0\\
1 & \delta &1-\delta&0\\
\hline
& \delta &1-\delta&0\\
 \end{array} \ \ \ \ \
\begin{array}{c|c c c}
0 & 0&0&0\\
\gamma & 0&\gamma&0\\
1 &0 &1-\gamma&\gamma\\
\hline
&0 &1-\gamma&\gamma\\
 \end{array}
\quad
\textrm{with}\; \gamma = 1-\frac{1}{\sqrt{2}}, \; \delta = 1-\frac{1}{2\gamma},
\end{displaymath}
and
\begin{displaymath}
\begin{array}{c|c c c c c}
0 & 0&0&0& 0 & 0\\
1/2 &1/2&0&0& 0 &0\\
2/3 &11/18&1/18&0& 0 &0\\
1/2 &5/6&-5/6&1/2& 0 &0\\
1 &1/4&7/4&3/4& -7/4 &0\\
\hline
&1/4&7/4&3/4& -7/4 &0\\
 \end{array} \ \ \ \ \
\begin{array}{c|c c c c c}
0 & 0&0&0& 0 & 0\\
1/2 &0&1/2&0&0 &0\\
2/3 &0&1/6&1/2& 0 &0\\
1/2 &0&-1/2&1/2& 1/2 &0\\
1 &0&3/2&-3/2& 1/2 &1/2\\
\hline
 &0&3/2&-3/2& 1/2 &1/2
 \end{array}~~.
\end{displaymath}
